# Supplementary material for: The interdependence between hospital choice and waiting time -- with a case study in urban China
Source: arXiv:2306.16256 source file (2023-06-28)
Supplement: Supplementary file 1 [file appendix2montecarloresults.pdf]

## Appendix 2

Base Base

| Probabilities | DCE Only | | | DCE & Queuing | | | Sign Test | Nonzero |
|---|---|---|---|---|---|---|---|---|
| *Pr(OO, M)* | 77.57 | 77.57 | | 77.59 | 77.40 | | -- | |
| *Pr(1, M)* | 07.84 | 07.84 | | 07.84 | 07.83 | | -- | |
| *Pr(2, M)* | 09.67 | 09.67 | | 09.66 | 09.72 | | PP | |
| *Pr(3, M)* | 04.92 | 04.92 | | 04.91 | 05.05 | | PP | |
| *Pr(OO, S)* | 00.06 | 00.06 | | 00.06 | 00.06 | | -- | |
| *Pr(1, S)* | 19.17 | 19.17 | | 19.18 | 19.06 | | -- | |
| *Pr(2, S)* | 27.09 | 27.09 | | 27.09 | 27.01 | | -- | |
| *Pr(3, S)* | 53.68 | 53.68 | | 53.67 | 53.87 | | PP | |
| | | | | | | | | |
| *W(1)* | 0.43 | 0.43 | | 0.43 | 0.43 | | -- | |
| *W(2)* | 1.53 | 1.50 | | 1.52 | 1.48 | | - | |
| *W(3)* | 3.54 | 3.58 | | 3.54 | 3.43 | | pp | |

Base Reduced Opt Out Utility

| Probabilities | DCE Only | | | DCE & Queuing | | | Sign Test | Nonzero |
|---|---|---|---|---|---|---|---|---|
| *Pr(OO, M)* | 49.80 | 49.80 | | 54.05 | 53.48 | | Pp | X |
| *Pr(1, M)* | 17.55 | 17.55 | | 18.59 | 18.44 | | Pp | X |
| *Pr(2, M)* | 21.64 | 21.64 | | 18.18 | 18.51 | | -- | X |
| *Pr(3, M)* | 11.01 | 11.01 | | 09.17 | 09.57 | | -- | |
| *Pr(OO, S)* | 00.06 | 00.06 | | 00.06 | 00.06 | | Pp | X |
| *Pr(1, S)* | 19.17 | 19.17 | | 20.79 | 20.53 | | Pp | X |
| *Pr(2, S)* | 27.09 | 27.09 | | 26.61 | 26.56 | | -- | |
| *Pr(3, S)* | 53.68 | 53.68 | | 52.54 | 52.85 | | -- | |
| | | | | | | | | |
| *W(1)* | 0.51 | 0.51 (739) | | 0.54 | 0.53 | | Pp | X |
| *W(2)* | 4.08 | 4.19 (739) | | 2.62 | 2.50 | | -- | X |
| *W(3)* | 6.92 | 5.24 (739) | | 4.66 | 4.46 | | -- | |

Base Increased Waiting Time Sensitivity

| Probabilities | DCE Only | | | DCE & Queuing | | | Sign Test | Nonzero |
|---|---|---|---|---|---|---|---|---|
| *Pr(OO, M)* | 77.57 | 77.57 | | 76.97 | 76.78 | | -- | X |
| *Pr(1, M)* | 07.84 | 07.84 | | 07.73 | 07.73 | | -- | X |
| *Pr(2, M)* | 09.67 | 09.67 | | 09.51 | 09.61 | | -- | |
| *Pr(3, M)* | 04.92 | 04.92 | | 05.77 | 05.88 | | PP | X |
| *Pr(OO, S)* | 00.06 | 00.06 | | 00.07 | 00.07 | | PP | X |
| *Pr(1, S)* | 19.17 | 19.17 | | 22.52 | 22.27 | | PP | X |
| *Pr(2, S)* | 27.09 | 27.09 | | 27.53 | 27.50 | | PP | |
| *Pr(3, S)* | 53.68 | 53.68 | | 49.86 | 50.15 | | -- | X |
| | | | | | | | | |
| *W(1)* | 0.43 | 0.43 | | 0.46 | 0.45 | | pp | X |
| *W(2)* | 1.52 | 1.48 | | 1.55 | 1.50 | | pp | |
| *W(3)* | 3.54 | 3.55 | | 2.80 | 2.72 | | -- | |

Medium Skill Base

| Probabilities | DCE Only | | | DCE & Queuing | | | Sign Test | Nonzero |
|---|---|---|---|---|---|---|---|---|
| *Pr(OO, M)* | 74.04 | 74.04 | | 74.11 | 73.90 | | -- | |
| *Pr(1, M)* | 12.04 | 12.04 | | 11.98 | 11.97 | | -- | |
| *Pr(2, M)* | 09.22 | 09.23 | | 09.24 | 09.31 | | PP | |
| *Pr(3, M)* | 04.70 | 04.70 | | 04.66 | 04.82 | | PP | |
| *Pr(OO, S)* | 00.06 | 00.06 | | 00.06 | 00.06 | | -- | |
| *Pr(1, S)* | 18.57 | 18.57 | | 18.57 | 18.42 | | -- | |
| *Pr(2, S)* | 27.29 | 27.29 | | 27.37 | 27.25 | | -- | |
| *Pr(3, S)* | 54.08 | 54.08 | | 54.00 | 54.27 | | PP | |
| | | | | | | | | |
| *W(1)* | 0.46 | 0.46 | | 0.46 | 0.45 | | -- | |
| *W(2)* | 1.51 | 1.48 | | 1.51 | 1.47 | | | |
| *W(3)* | 3.60 | 3.59 | | 3.57 | 3.43 | | pp | |

Medium Skill Reduced Opt Out Utility

| Probabilities | DCE Only | | | DCE & Queuing | | | Sign Test | Non Zero |
|---|---|---|---|---|---|---|---|---|
| *Pr(OO, M)* | 44.99 | 44.99 | | 48.38 | 47.90 | | Pp | X |
| *Pr(1, M)* | 25.52 | 25.52 | | 26.28 | 26.11 | | Pp | |
| *Pr(2, M)* | 19.55 | 19.55 | | 16.93 | 18.51 | | -- | X |
| *Pr(3, M)* | 09.95 | 09.95 | | 08.40 | 08.77 | | -- | |
| *Pr(OO, S)* | 00.06 | 00.06 | | 00.06 | 00.06 | | Pp | X |
| *Pr(1, S)* | 18.57 | 18.57 | | 19.83 | 19.60 | | Pp | X |
| *Pr(2, S)* | 27.29 | 27.29 | | 27.05 | 26.98 | | -- | |
| *Pr(3, S)* | 54.08 | 54.08 | | 53.05 | 53.36 | | - | |
| | | | | | | | | |
| *W(1)* | 0.59 | 0.58 (785) | | 0.62 | 0.61 | | Pp | X |
| *W(2)* | 3.23 | 3.21 (785) | | 2.45 | 2.34 | | -- | X |
| *W(3)* | 6.30 | 5.01 (785) | | 4.56 | 4.37 | | -- | |

Medium Skill Increased Waiting Time Sensitivity

| Probabilities | DCE Only | | | DCE & Queuing | | | Sign Test | Nonzero |
|---|---|---|---|---|---|---|---|---|
| *gPr(OO, M)* | 74.04 | 74.04 | | 73.58 | 73.39 | | -- | |
| *Pr(1, M)* | 12.04 | 12.04 | | 11.83 | 11.81 | | -- | X |
| *Pr(2, M)* | 09.22 | 09.23 | | 09.10 | 09.18 | | - | |
| *Pr(3, M)* | 04.70 | 04.70 | | 05.49 | 05.61 | | PP | X |
| *Pr(OO, S)* | 00.06 | 00.06 | | 00.08 | 00.07 | | PP | X |
| *Pr(1, S)* | 18.57 | 18.57 | | 21.80 | 21.52 | | PP | X |
| *Pr(2, S)* | 27.29 | 27.29 | | 27.89 | 27.79 | | PP | |
| *Pr(3, S)* | 54.08 | 54.08 | | 50.23 | 50.62 | | -- | X |
| | | | | | | | | |
| *W(1)* | 0.46 | 0.46 | | 0.49 | 0.48 | | Pp | X |
| *W(2)* | 1.51 | 1.47 | | 1.55 | 1.50 | | Pp | |
| *W(3)* | 3.60 | 3.55 | | 2.82 | 2.73 | | -- | X |

Expert Skill Base

| Probabilities | DCE Only | | | DCE & Queuing | | | Sign Test | Nonzero |
|---|---|---|---|---|---|---|---|---|
| *Pr(OO, M)* | 75.87 | 75.87 | | 75.45 | 75.26 | | -- | |
| *Pr(1, M)* | 10.94 | 10.94 | | 10.80 | 10.79 | | -- | |
| *Pr(2, M)* | 08.38 | 08.38 | | 08.14 | 08.22 | | -- | |
| *Pr(3, M)* | 04.81 | 04.81 | | 05.60 | 05.73 | | PP | X |
| *Pr(OO, S)* | 00.05 | 00.05 | | 00.05 | 00.05 | | -- | |
| *Pr(1, S)* | 20.87 | 20.87 | | 20.20 | 20.09 | | -- | X |
| *Pr(2, S)* | 30.68 | 30.68 | | 29.49 | 29.44 | | -- | X |
| *Pr(3, S)* | 48.40 | 48.40 | | 50.26 | 50.42 | | Pp | X |
| | | | | | | | | |
| *W(1)* | 0.47 | 0.47 | | 0.46 | 0.46 | | -- | X |
| *W(2)* | 1.77 | 1.72 | | 1.62 | 1.57 | | -- | X |
| *W(3)* | 2.41 | 2.36 | | 2.85 | 2.76 | | Pp | X |

Expert Skill Reduced Opt Out Utility

| Probabilities | DCE Only | | | DCE & Queuing | | | Sign Test | Nonzero |
|---|---|---|---|---|---|---|---|---|
| *Pr(OO, M)* | 47.42 | 47.42 | | 50.18 | 49.81 | | Pp | X |
| *Pr(1, M)* | 23.83 | 23.83 | | 24.18 | 24.07 | | -- | |
| *Pr(2, M)* | 18.26 | 18.26 | | 15.21 | 15.43 | | -- | X |
| *Pr(3, M)* | 10.49 | 10.49 | | 10.42 | 10.69 | | PP | |
| *Pr(OO, S)* | 00.05 | 00.06 | | 00.06 | 00.06 | | Pp | |
| *Pr(1, S)* | 20.87 | 20.87 | | 21.50 | 21.33 | | Pp | |
| *Pr(2, S)* | 30.68 | 30.68 | | 29.04 | 29.03 | | -- | X |
| *Pr(3, S)* | 48.40 | 48.40 | | 49.41 | 49.58 | | -- | |
| | | | | | | | | |
| *W(1)* | 0.60 | 0.60 (925) | | 0.62 | 0.61 | | Pp | |
| *W(2)* | 4.40 | 4.31 (925) | | 2.55 | 2.46 | | -- | X |
| *W(3)* | 3.49 | 3.49 (925) | | 3.80 | 3.67 | | -- | |

Expert Skill Increased Waiting Time Sensitivity

| Probabilities | DCE Only | | | DCE & Queuing | | | Sign Test | Nonzero |
|---|---|---|---|---|---|---|---|---|
| *Pr(OO, M)* | 75.87 | 75.87 | | 75.04 | 74.89 | | -- | X |
| *Pr(1, M)* | 10.94 | 10.94 | | 10.68 | 10.67 | | -- | X |
| *Pr(2, M)* | 08.38 | 08.38 | | 08.11 | 08.18 | | -- | |
| *Pr(3, M)* | 04.81 | 04.81 | | 06.17 | 06.26 | | PP | X |
| *Pr(OO, S)* | 00.05 | 00.05 | | 00.06 | 00.06 | | Pp | X |
| *Pr(1, S)* | 20.87 | 20.87 | | 23.33 | 23.10 | | Pp | X |
| *Pr(2, S)* | 30.66 | 30.68 | | 29.46 | 29.44 | | -- | |
| *Pr(3, S)* | 48.40 | 48.40 | | 47.15 | 47.39 | | -- | |
| | | | | | | | | |
| *W(1)* | 0.47 | 0.47 | | 0.47 | 0.48 | | pp | X |
| *W(2)* | 1.77 | 1.73 | | 1.61 | 1.56 | | - | |
| *W(3)* | 2.41 | 2.36 | | 2.41 | 2.34 | | pp | |

Upgrade Equipment Base

| Probabilities | DCE Only | | | DCE & Queuing | | | Sign Test | Nonzero |
|---|---|---|---|---|---|---|---|---|
| *Pr(OO, M)* | 71.29 | 71.29 | | 70.46 | 70.29 | | -- | X |
| *Pr(1, M)* | 12.49 | 12.49 | | 11.94 | 11.93 | | -- | X |
| *Pr(2, M)* | 11.70 | 11.70 | | 11.10 | 11.10 | | -- | |
| *Pr(3, M)* | 04.52 | 04.52 | | 06.50 | 06.57 | | PP | X |
| *Pr(OO, S)* | 00.04 | 00.04 | | 00.04 | 00.04 | | -- | X |
| *Pr(1, S)* | 32.20 | 32.20 | | 30.03 | 29.94 | | -- | X |
| *Pr(2, S)* | 29.60 | 29.60 | | 27.52 | 27.55 | | -- | X |
| *Pr(3, S)* | 38.16 | 38.16 | | 42.41 | 42.47 | | PP | X |
| | | | | | | | | |
| *W(1)* | 0.62 | 0.61 | | 0.58 | 0.57 | | -- | X |
| *W(2)* | 2.03 | 1.98 | | 1.69 | 1.65 | | - | X |
| *W(3)* | 1.49 | 1.46 | | 1.91 | 1.86 | | pp | X |

Advanced Equipment Reduced Opt Out Utility

| Probabilities | DCE Only | | | DCE & Queuing | | | Sign Test | Nonzero |
|---|---|---|---|---|---|---|---|---|
| *Pr(OO, M)* | | 41.60 | | 44.10 | 43.79 | | Pp | X |
| *Pr(1, M)* | | 25.41 | | 24.67 | 24.61 | | -- | X |
| *Pr(2, M)* | | 23.80 | | 18.97 | 19.20 | | -- | X |
| *Pr(3, M)* | | 09.20 | | 12.27 | 12.40 | | PP | X |
| *Pr(OO, S)* | | 00.04 | | 00.04 | 00.04 | | -- | |
| *Pr(1, S)* | | 32.20 | | 31.20 | 31.09 | | -- | X |
| *Pr(2, S)* | | 29.60 | | 26.36 | 26.41 | | -- | X |
| *Pr(3, S)* | | 38.16 | | 42.39 | 42.44 | | PP | X |
| | Infeasible | | | | | | | |
| *W(1)* | | 0.84 (530) | | 0.81 | 0.79 | | -- | X |
| *W(2)* | | 5.63 (530) | | 2.75 | 2.66 | | - | X |
| *W(3)* | | 1.72 (530) | | 2.54 | 2.47 | | pp | X |

Upgrade Equipment Increased Waiting Time Sensitivity

| Probabilities | DCE Only | | | DCE & Queuing | | | Sign Test | Nonzero |
|---|---|---|---|---|---|---|---|---|
| *Pr(OO, M)* | 71.29 | 71.29 | | 70.24 | 70.09 | | -- | X |
| *Pr(1, M)* | 12.49 | 12.49 | | 11.80 | 11.80 | | -- | X |
| *Pr(2, M)* | 11.70 | 11.70 | | 11.26 | 11.36 | | -- | |
| *Pr(3, M)* | 04.52 | 04.52 | | 06.70 | 06.75 | | PP | X |
| *Pr(OO, S)* | 00.04 | 00.04 | | 00.04 | 00.04 | | PP | X |
| *Pr(1, S)* | 32.20 | 32.20 | | 32.81 | 32.64 | | PP | |
| *Pr(2, S)* | 29.60 | 29.60 | | 26.63 | 26.72 | | -- | X |
| *Pr(3, S)* | 38.16 | 38.16 | | 40.51 | 40.59 | | PP | X |
| | | | | | | | | |
| *W(1)* | 0.62 | 0.61 | | 0.62 | 0.61 | | -- | |
| *W(2)* | 2.03 | 1.97 | | 1.62 | 1.57 | | - | X |
| *W(3)* | 1.49 | 1.46 | | 1.77 | 1.73 | | pp | X |

Upskill and Upgrade Base

| Probabilities | DCE Only | | | DCE & Queuing | | | Sign Test | Nonzero |
|---|---|---|---|---|---|---|---|---|
| *Pr(OO, M)* | 68.56 | 68.56 | | 67.91 | 67.76 | | -- | X |
| *Pr(1, M)* | 17.13 | 17.13 | | 16.11 | 16.11 | | -- | X |
| *Pr(2, M)* | 09.97 | 09.97 | | 09.27 | 09.38 | | -- | X |
| *Pr(3, M)* | 04.35 | 04.35 | | 06.71 | 06.76 | | PP | X |
| *Pr(OO, S)* | 00.03 | 00.04 | | 00.04 | 00.04 | | -- | X |
| *Pr(1, S)* | 34.03 | 34.03 | | 31.58 | 31.51 | | -- | X |
| *Pr(2, S)* | 32.54 | 32.54 | | 30.05 | 30.11 | | -- | X |
| *Pr(3, S)* | 33.39 | 33.39 | | 38.33 | 38.34 | | PP | X |
| | | | | | | | | |
| *W(1)* | 0.72 | 0.71 | | 0.66 | 0.65 | | -- | X |
| *W(2)* | 2.26 | 2.20 | | 1.79 | 1.73 | | - | X |
| *W(3)* | 1.26 | 1.24 | | 1.61 | 1.58 | | pp | X |

Upskill and Upgrade Reduced Opt Out Utility

| Probabilities | DCE Only | | | DCE & Queuing | | | Sign Test | Nonzero |
|---|---|---|---|---|---|---|---|---|
| *Pr(OO, M)* | 38.47 | 38.47 | | 40.78 | 40.42 | | Pp | X |
| *Pr(1, M)* | 33.52 | 33.52 | | 30.88 | 30.86 | | -- | X |
| *Pr(2, M)* | 19.50 | 19.50 | | 15.76 | 16.03 | | -- | X |
| *Pr(3, M)* | 08.51 | 08.51 | | 12.58 | 12.68 | | PP | X |
| *Pr(OO, S)* | 00.04 | 00.04 | | 00.04 | 00.04 | | -- | |
| *Pr(1, S)* | 34.03 | 34.03 | | 32.18 | 32.07 | | -- | X |
| *Pr(2, S)* | 32.54 | 32.54 | | 29.09 | 29.20 | | -- | X |
| *Pr(3, S)* | 33.39 | 33.39 | | 38.69 | 38.69 | | PP | X |
| | | | | | | | | |
| *W(1)* | 1.26 | 1.23 (660) | | 1.04 | 1.00 | | -- | X |
| *W(2)* | 8.70 | 5.11 (660) | | 2.69 | 2.58 | | - | X |
| *W(3)* | 1.43 | 1.40 (660) | | 2.09 | 2.02 | | pp | X |

Upskill and Upgrade Increased Waiting Time Sensitivity

| | | | | | | | | |
|---|---|---|---|---|---|---|---|---|
| *Pr(OO, M)* | 68.56 | 68.56 | | 67.68 | 67.63 | | -- | X |
| *Pr(1, M)* | 17.13 | 17.13 | | 15.93 | 15.95 | | -- | X |
| *Pr(2, M)* | 09.97 | 09.97 | | 09.50 | 09.58 | | -- | |
| *Pr(3, M)* | 04.35 | 04.35 | | 06.80 | 06.84 | | PP | X |
| *Pr(OO, S)* | 00.04 | 00.04 | | 00.04 | 00.04 | | Pp | X |
| *Pr(1, S)* | 34.03 | 34.03 | | 33.94 | 33.81 | | -- | |
| *Pr(2, S)* | 32.54 | 32.54 | | 28.82 | 28.92 | | -- | X |
| *Pr(3, S)* | 33.39 | 33.39 | | 37.19 | 37.23 | | PP | X |
| | | | | | | | | |
| *W(1)* | 0.72 | 0.71 | | 0.70 | 0.68 | | -- | X |
| *W(2)* | 2.26 | 2.21 | | 1.67 | 1.63 | | - | X |
| *W(3)* | 1.26 | 1.24 | | 1.55 | 1.51 | | pp | X |
